# Supplementary material for: On the Performance of Reed-Muller Codes Over $(d,\infty)$-RLL Input-Constrained BMS Channels
Source: arXiv:2201.02035 source file (2022-01-06)
Supplement: Supplementary file 1 [file AppendixA.tex]

Proposition \ref{prop:simplify} simplifies the maximizing values $\vec{\delta}^*:=(\delta_0^*,\ldots,\delta_d^*)$ in the two cases when the maximum is attained at an interior point of $\Delta_d$ and when it is attained on the boundary.

First, we characterize the stationary points of $R(\vec{\delta})$. We define
\begin{align*}
	N(\vec{\delta})&:=\bar{\epsilon}\left(\sum_{i=0}^{d}\epsilon^i h_b(\delta_i)\right),\ \text{and}\\
	D(\vec{\delta})&:=\sum_{i=0}^{d}\epsilon^i + d\bar{\epsilon}\left(\sum_{i=0}^{d}\epsilon^i\delta_i\right),
\end{align*}
to be the numerator and the denominator of $R(\vec{\delta})$, respectively. Note that for any $i\in [0:d]$,
\begin{align}
\frac{\partial R(\vec{\delta})}{\partial \delta_i}\Biggr|_{\vec{\delta} = \vec{\tilde{\delta}}} = 0 &\implies \bar{\epsilon}\epsilon^i\log_2\left(\frac{1-{\tilde{\delta}_i}}{\tilde{\delta}_i}\right)\cdot D(\vec{\tilde{\delta}}) = d\bar{\epsilon}\epsilon^i\cdot N(\vec{\tilde{\delta}}) \notag\\
&\implies \frac{N(\vec{\tilde{\delta}})}{D(\vec{\tilde{\delta}})} = \frac{1}{d}\log_2\left(\frac{1-\tilde{\delta_i}}{\tilde{\delta}_i}\right) \label{eq:maximizer}.
\end{align}
Therefore, from \eqref{eq:maximizer}, we get that
\[
\frac{\partial R(\vec{\delta})}{\partial \delta_i}\Biggr|_{\vec{\delta} = \vec{\tilde{\delta}}} = 0, \forall i\ \implies \tilde{\delta}_0 = \ldots = \tilde{\delta}_d.
\]
Thus, when the maximum in \eqref{eq:fbcap} is attained at an interior point, it holds that $\delta_0^* = \ldots =\delta_d^* =\delta^*$, thereby showing that in the first case, the feedback capacity
\[
C_{(d,\infty)}^{\text{fb}}(\epsilon) = \max_{\delta\in [0,\frac{1}{d+1}]} \frac{h_b(\delta)}{d\delta + \frac{1}{1-\epsilon}}.
\]
If the maximum is attained at a boundary point of $\Delta_d$, we wish to show that it holds that $\sum_{i=0}^{d}\delta_i^* = 1$. To this end, we first the define the following non-linear optimization problem with affine constraints:
\begin{align}
	&\text{\textbf{maximize}}\ R(\delta_0,\ldots,\delta_d) \notag\\
	&\text{\textbf{subj. to}}\ g_0(\vec{\delta}) := -\delta_0\leq 0,\ldots, g_d(\vec{\delta}) := -\delta_d\leq 0, \notag \\
	&\ \ \ \ \ \ \ \ \ \ \tilde{g}_0(\vec{\delta}) := \delta_0-1\leq 0,\ldots, \tilde{g}_d(\vec{\delta}) := \delta_d-1\leq 0, \notag\\
	&\ \ \ \ \ \ \ \ \ \ \ \ \ \ \ \ \ \ \hat{g}(\vec{\delta}) := \delta_0+\ldots+\delta_d - 1\leq 0. \label{eq:opt1}
\end{align}

Note that the objective function in \eqref{eq:opt1} and the constraint functions are all continuously differentiable in $[0,1]^{d+1}$ and the constraints are affine functions. Therefore, it holds from the necessity of the Karush-Kuhn-Tucker (KKT) conditions being satisfied, that there exist constants $\{\mu_i\}_{i=0}^{d}$, $\{\tilde{\mu}_i\}_{i=0}^{d}$, and $\hat{\mu}$, with $\mu_i, \tilde{\mu}_i \geq 0, \ \forall i$, and $\hat{\mu}\geq 0$, such that:
\begin{align}
	\label{eq:opt2}
\nabla R(\vec{\delta}) \Big|_{\vec{\delta} = \vec{\delta}^*} = \left(\sum_{i=0}^{d}\mu_i\nabla g_i(\vec{\delta})+\sum_{i=0}^{d}\tilde{\mu}_i\nabla \tilde{g}_i(\vec{\delta})+\hat{\mu}\nabla \hat{g}(\vec{\delta})\right)\Bigg|_{\vec{\delta} = \vec{\delta}^*}.
\end{align}
Suppose that the maximum is attained at a boundary point with $\delta_j^* = 0$, for some $j\in [0:d]$. Following reasoning similar to that in Lemma 13 in Appendix A of \cite{0k}, we note that since $\delta_j^* = 0$, we do not need to worry about the constraint that $\tilde{g}_j(\vec{\delta}) \leq 0$. Equation \eqref{eq:opt2} then gives us:
\[
\frac{\partial R(\vec{\delta})}{\partial \delta_j}\Biggr|_{\delta_j = 0} = -\mu_j + \hat{\mu}.
\]
However, we note that the left side of the equation above is
\[
\frac{\partial R(\vec{\delta})}{\partial \delta_j}\Biggr|_{\delta_j = 0} = \frac{\bar{\epsilon}\epsilon^i\log_2\left(\frac{1-{\tilde{\delta}_i}}{\tilde{\delta}_i}\right)\cdot D(\vec{\delta}) - d\bar{\epsilon}\epsilon^i\cdot N(\vec{\delta})}{\left(D(\vec{\delta})\right)^2},
\]
which tends to $+\infty$ as $\delta \to 0^+$. Therefore, it must be that $\hat{\mu}=+\infty$. 

Now, again, since the KKT conditions are necessary conditions for optimality in our maximization problem, from the complementary slackness condition, we see that:
\begin{align}
	\label{eq:opt3}
\hat{\mu}\hat{g}(\vec{\delta}^*)+\sum_{i=0}^{d}\mu_ig_i(\vec{\delta}^*)+\sum_{i=0}^{d}\tilde{\mu}_i\tilde{g}_i(\vec{\delta}^*) = 0.
\end{align}
From the fact that $\hat{\mu} = +\infty$ when the maximum is attained at a boundary point, it follows from equation \eqref{eq:opt3} that $\hat{g}(\vec{\delta}^*) = 0$, or, that $\sum_{i=0}^{d}\delta^*_i = 0$ when $\delta_j=0$ for some $j$.
